# Supplementary material for: All-Norm Load Balancing in Graph Streams via the Multiplicative Weights Update Method
Source: arXiv:2301.07007 source file (2023-01-17)
Supplement: Supplementary file 1 [file appendix.tex]

\part*{Appendix: Omitted Simple Proofs}

\begin{proof}[Proof of \Cref{lem:merge-size}]
  The algorithm guarantees that $\tx$ is always a $(\kappa, \tau)$-matching.
  That $\tx \ge x$ is also clear; $\tx$ is initialized to $x$ and only
  increases from then on.

  Let us now show that $2\tx(E) \ge y(E)$.
  Let $T = \{ v \in V : \tx(v) = b(v) \}$ be the set of $\tx$-saturated
  vertices, and let $F = \{ uv \in E : u \not\in T \wedge v \not\in T\}$ be
  the set of edges with neither endpoint $\tx$-saturated.

  We will show that $y(F) \le \tx(F)$ and $y(E \setminus F) \le 2\tx(E \setminus F)$, which establishes that $y(E) \le 2\tx(E)$.
  The first inequality follows quickly:
  For $e \in F$, the value of $\tx(e)$ was raised to $x(e) + y(e)$,
  and hence $y(e) \le \tx(e)$.
  Now we bound $y(E \setminus F)$.
  Notice that for $v \in T$ we have $y(\delta(v)) \le b(v) = \tx(\delta(v))$,
  and hence
    \begin{align*}
        \sum_{e \in E\setminus F} y(e) &\le \sum_{v \in T} y(\delta(v))\\
            &\le \sum_{v \in T} \tx(\delta(v))\\
            &\le 2 \sum_{e \in E \setminus F} \tx(e). \qedhere
    \end{align*}
\end{proof}
